# Supplementary material for: LLM2Vec: Large Language Models Are Secretly Powerful Text Encoders
Source: arXiv:2404.05961 source file (2024-08-21)
Supplement: Supplementary file 1 [file legacy_appendix.tex]

\section{Data for plotting zeroshot perfromance using TSNE}\label{app:zeroshot_custom_reviews}
We report the data samples used in manual inspection of zeroshot models in \Cref{fig:mistral_zero_shot_pooling_qualitative} in \Cref{tab:custom-zeroshot-ablation}. Moreover, we exemplify the tasks used in our analysis of \Cref{fig:mistral_ret_cls_qualitative} in \Cref{tab:tsne-ret-cls}.

\begin{table}[]
    \centering
    \begin{tabular}{ll}
    \toprule
    Category & Task \\ \toprule
    \multicolumn{1}{l}{\multirow{3}{*}{Retrieval}} & SciFact\\
    & ArguAna\\
    & NFCorpus\\ \midrule
    
    \multicolumn{1}{l}{\multirow{2}{*}{Reranking}} & SciDocsRR\\
    & StackOverflowDupQuestions\\ \midrule

    \multicolumn{1}{l}{\multirow{3}{*}{Clustering}} & BiorxivClusteringS2S\\
    & MedrxivClusteringS2S\\ 
    & TwentyNewsgroupsClustering \\ \midrule

    \multicolumn{1}{l}{\multirow{1}{*}{Pair Classification}} & SprintDuplicateQuestions\\ \midrule

    \multicolumn{1}{l}{\multirow{3}{*}{Classification}} & Banking77Classification\\
    & EmotionClassification\\ 
    & MassiveIntentClassification \\ \midrule

    \multicolumn{1}{l}{\multirow{3}{*}{STS}} & STS17\\
    & SICK-R\\ 
    & STSBenchmark \\
    \bottomrule
    \end{tabular}
    \caption{The subset of MTEB evaluation benchmark used in plots and ablation studies.}
    \label{tab:mteb-subset}
\end{table}
\section{Evaluation subset} \label{app:mteb-subset}
We conduct some of the ablations and experiments for plotting on only a subset of 15 tasks of MTEB. The list of tasks is presented in \Cref{tab:mteb-subset}

\begin{table*}[t]
    \centering
    \begin{tabular}{c c p{12cm}}
    \toprule
       Category & Label & Review \\\midrule
       
       Movie & Negative & Poor Things simply just wasn't for me. I really don't like to say I hate a movie... so we'll just go with \"it wasn't for me\". I did appreciate the production design and performances, but a lot of the cinematography and writing/directing choices just didn't work for me. Just a little too weird for my tastes. And felt way too long. I wanted to like it so bad, and was so disappointed to find myself disliking it so much. I know it's been getting good reviews from most people - I'm in the minority here! So if you're interested, definitely check it out! I'm a huge supporter of going to see a film if you are interested in it and deciding for yourself how you feel!\\\midrule
       
       Movie & Positive & I saw this yesterday along with several other movies, that's why I'm reviewing the next day. Poor Things is very well-made, smoothly written throughout, with excellent cinematography, and a rivetingly bizarre experience that is so worthy of award recognition! It is dystopian vibe reminds me of Terry Gilliam's style. Yorgos is exceptional at his craft involving surgical creations, color palettes different from most, and enriching dialogue that is clever yet sometimes weird in all his movies. Emma Stone deserves praise and Willem Dafoe is master class as always. The film might not be for everyone but it's surely impressive and deserving of the 8.5 rating.\\\midrule

       Phone & Negative & Own an Apple 11 mini, broke the screen and forgot my passcode to my apple ID. So here is where the problems start, can't reset passcode because they want to send a verification code to my phone, which is now broken. Can't set a different phone to receive my verification and when given a code by email it sends a link to apple.com at which point I need to sign in to my account to input verification code, which I have no passcode for so have no access to. When I hit reset passcode the cycle begins again. So even if I get a new iPhone I can't use it because it won't accept service until I sign into my account, which I can't because I don't have passcode, and they will only send passcode to my broken phone, and the cycle repeats.\\\midrule

       Phone & Positive & The iPhone 11 is a big surprise, packing more advanced technology (namely in the camera capabilities and the processing power under the hood) at a lower cost than the iPhone XR's price in 2018. It combines a large 6.1-inch display with a premium-feeling body, and comes in an array of colors too.\\\bottomrule
       \toprule
       \multicolumn{2}{c}{Category} & \multicolumn{1}{l}{Instruction} \\\midrule
       \multicolumn{2}{c}{Classification} & \multicolumn{1}{l}{Represent the sentence for classification:} \\
       \multicolumn{2}{c}{STS} & \multicolumn{1}{l}{Represent the sentence for semantic textual similarity:} \\
       \bottomrule
    \end{tabular}
    \caption{The four reviews and instructions for the TSNE visualization. Instruction categories include Classification, STS, and no instruction.}
    \label{tab:custom-zeroshot-ablation}
\end{table*}

\begin{table*}[t]
    \centering
    \begin{tabular}{c c p{12cm}}
    \toprule
       Task & Type & Text \\\midrule
       
       Retrieval & Query & Represent the medicine question for retrieving relevant documents; New daily persistent headache: should migrainous features be incorporated?\\\midrule
       
       Retrieval & Document & Represent the medicine document for retrieval; International Classification of Headache Disorders (ICHD-2) criteria for new daily persistent headache (NDPH) require tension-type headache features. Many patients with 'new-onset persistent' headache fail to fulfil such criteria due to prominent migrainous features.We reviewed all NDPH patients in our headache clinic, using the definition of persistent headache < 3 days after onset for > 3 months. The patients were dichotomised: patients meeting ICHD-2 criteria (NDPH-S) and patients failing to meet ICHD-2 criteria due to prominent migrainous features (NDPH-M). All patients had completed a structured intake form including demographics, headache profiles, Beck Depression Inventory (BDI), Short Form 36 (SF-36) Health Survey, and Migraine Disability Assessment (MIDAS). A telephone interview was conducted for follow-up.A total of 92 NDPH patients were enrolled (59 (64.1\%) NDPH-M, 33 (35.9\%) NDPH-S). Between the two subgroups, the sociodemographics were indistinguishable, but the patients with NDPH-M had higher headache intensity, BDI scores, MIDAS scores, and lower scores of most SF-36 subscales. After an average of 2 years of follow-up, 57 (66\%) had a good outcome ($\geq$ 50\% reduction in headache frequency). Cox proportional analysis showed that disease duration $\leq$6 months and NDPH-S diagnosis predicted good outcomes.\\\midrule
       
       Classification & Query & Represent this sentence for classification: When it works, its awesome. But mine died after about 8 months of normal use. The thing is, its under warranty and they won't repair it, since we bought through amazon. And you only have 90 days.\\\midrule

       Classification & Document & Represent this sentence for classification: Not even 6 months and it no longer works. Just out of warranty. I tried to contact HP by email for warranty service but they weren't helpful. For now, I'll shell out more than \$250 at Best Buy - which includes an extended warrenty.\\
       \bottomrule
    \end{tabular}
    \caption{Examples of retrieval (pubmed) and classification (roducts reviews classification) datasets with corresponding instruction.}
    \label{tab:tsne-ret-cls}
\end{table*}

\section{Detailed results}
Put a table of all detailed results for models

\section{Representation space visualizations}

%--------------------------------------
\begin{figure*}[t]
    \centering
    \includegraphics[width=0.28\linewidth]{Plots/TSNE/custom zeroshot eos causal - no legend.pdf}
    \includegraphics[width=0.28\linewidth]{Plots/TSNE/custom zeroshot eos bidirectional - no legend.pdf}
    \includegraphics[width=0.41\linewidth]{Plots/TSNE/custom zeroshot mean bidirectional.pdf}
    \caption{Zero shot performance of Mistral given different instructions and reviews. Reviews are available in \Cref{app:zeroshot_custom_reviews}.}
    \label{fig:mistral_zero_shot_pooling_qualitative}
\end{figure*}
%--------------------------------------

%--------------------------------------
\begin{figure*}[t]
    \centering
    \includegraphics[width=0.26\linewidth]{Plots/TSNE/mixed zeroshot eos causal - no legend.pdf}
    \includegraphics[width=0.26\linewidth]{Plots/TSNE/mixed zeroshot mean bidirectional - no legend.pdf}
    \includegraphics[width=0.44\linewidth]{Plots/TSNE/mixed trained mean bidirectional.pdf}
    \caption{Caption. \parishadsuggests{}{should be recreated with mlm results maybe.}}
    \label{fig:mistral_ret_cls_qualitative}
\end{figure*}
%--------------------------------------

\begin{table*}[ht]
    \centering
    \small
    \begin{tabular}{lccccccccc}
    \toprule
    \multicolumn{1}{l}{\multirow{2}{*}{\# of datasets $\rightarrow$}} & Retr. & Rerank. & Clust. & PairClass. & Class. & STS & Avg\\
    \multicolumn{1}{l}{}                                & 3     & 2     & 3          & 1      & 3    & 3    & 15  \\
    \midrule
    \multicolumn{1}{l}{medi-ml-miracl bi mean}  & 58.05  & 71.08  & 42.93  &  92.07  & 69.68  & 85.76 & \textbf{66.90} \\
    \midrule
    \multicolumn{9}{l}{\emph{Connections and Pooling}}        \\ \midrule
    \multicolumn{1}{l}{mistral medi-ml-miracl bi eos} & 58.77 & 71.1 & 43.55 & 85.3 & 69.57 & 85.87 & 66.72 \\
    \multicolumn{1}{l}{mistral medi-ml-miracl bi w-mean}  & 57.96 & 70.96 & 42.94 & 92.24 & 69.91 & 85.49 & 66.87 \\ 
    \multicolumn{1}{l}{mistral medi-ml-miracl uni eos}  & 58.35 & 70.62 & 42.76 & 88.96 & 69.52 & 85.87 & 66.65\\ 
    \multicolumn{1}{l}{mistral medi-ml-miracl uni mean}  & 56.81 & 70.55 & 41.48 & 88.91 & 70.72 & 84.82 & 66.1 \\ 
    \multicolumn{1}{l}{mistral medi-ml-miracl uni w-mean}  & 56.81 & 70.53 & 41.42 & 90.15 & 70.79 & 85.42 & 66.3 \\ 
    \midrule
    \multicolumn{9}{l}{\emph{Instruction-tuned}}        \\ \midrule
    \multicolumn{1}{l}{no-instruct medi-ml-miracl bi mean} & 58.28 & 71.71 & 42.82 & 94.2 & 69.26 & 83.14 & 66.54 & \\
    \midrule
    \multicolumn{9}{l}{\emph{Hyperparameters}}        \\ \midrule
    \multicolumn{1}{l}{mistral medi-ml-miracl bi mean lora\_r-8} & 57.92 & 71.03 & 43.4 & 91.42 & 69.69 & 85.6 & 66.89\\
    \multicolumn{1}{l}{mistral medi-ml-miracl bi mean lora\_r-32} & 58.08 & 71.04 & 42.55 & 91.67 & 70.76 & 85.61 & 66.98\\
    \multicolumn{1}{l}{mistral medi-ml-miracl bi mean bs-256} & 58.12 & 70.52 & 42.72 & 83.57 & 69.44 & 84.32 & 65.89\\
    \multicolumn{1}{l}{mistral medi-ml-miracl bi mean bs-512} & 57.55 & 70.5 & 41.77 & 80.79 & 68.57 & 84.36 & 65.24\\
    \midrule
    \multicolumn{9}{l}{\emph{Training Data}}        \\ \midrule
    \multicolumn{1}{l}{mistral medi-eng-miracl bi mean} & 57.41 & 71.09 & 42.55 & 81.44 & 69.42 & 85.21 & 65.83 \\
    \multicolumn{1}{l}{mistral medi bi mean} & 57.6 & 70.61 & 43.24 & 91.57 & 70.11 & 85.27 & 66.76 \\
    \bottomrule
    \end{tabular}
    \caption{Dummy caption for ablation table, all without MLM. mistral-7b: \{uni,bi\}, pool\{mean,eos,weighted\}, \{inst,no-inst\}, bs\{256,512\}, lora{8, 32}. \parishadsuggests{}{This table goes to the appendix and another one with MLM models comes instead.}}
    \label{tab:ablation_results_no_mlm}
\end{table*}

\begin{table*}[ht]
    \centering
    \small
    \begin{tabular}{lccccccccc}
    \toprule
    % \multicolumn{1}{l}{\multirow{2}{*}{\# of datasets $\rightarrow$}} & Class. & Clust. & PairClass. & Rerank & Retr. & STS & Summ. & Avg \\
    % \multicolumn{1}{l}{}                                & 12     & 11     & 3          & 4      & 15    & 10  & 1    & 56  \\
    \multicolumn{1}{l}{\multirow{2}{*}{\# of datasets $\rightarrow$}} & Retr. & Rerank. & Clust. & PairClass. & Class. & STS & Avg\\
    \multicolumn{1}{l}{}                                & 3     & 2     & 3          & 1      & 3    & 3    & 15  \\ 
    \midrule
    % \multicolumn{9}{l}{\emph{Training Data}}        \\ \cmidrule{1-1}
    \multicolumn{1}{l}{medi-ml-miracl}  & 58.05  & 71.08  & 42.93  &  92.07  & 69.68  & 85.76 & \textbf{66.90} \\
    \multicolumn{1}{l}{medi-eng-miracl} & 57.41 & 71.09 & 42.55 & 81.44 & 69.42 & 85.21 & 65.83\\
    \multicolumn{1}{l}{medi} & 57.6 & 70.61 & 43.24 & 91.57 & 70.11 & 85.27 & 66.76\\
    \bottomrule
    \end{tabular}
    \caption{Ablation study of the impact of training data on Mistral-7B on MTEB benchmark (bi-mean Mistral-7b with no MLM training).}
    \label{tab:training-data-ablation}
\end{table*}
