# Supplementary material for: LLM2Vec: Large Language Models Are Secretly Powerful Text Encoders
Source: arXiv:2404.05961 source file (2024-08-21)
Supplement: Supplementary file 2 [file future_work.tex]

%--------------------------------------
\section{Future work}
\label{sec:appendix:future_work}
%--------------------------------------

\mm{Collect ideas for future work here.}
