# Supplementary material for: LLM2Vec: Large Language Models Are Secretly Powerful Text Encoders
Source: arXiv:2404.05961 source file (2024-08-21)
Supplement: Supplementary file 3 [file more_llm2vec.tex]

%--------------------------------------
\newpage
\section{More details on our implementation of LLM2Vec}
\label{sec:appendix:llm2vec}
%--------------------------------------

\mm{Provide LLM2Vec details here.}
