# Supplementary material for: LLM2Vec: Large Language Models Are Secretly Powerful Text Encoders
Source: arXiv:2404.05961 source file (2024-08-21)
Supplement: Supplementary file 4 [file more_related_work.tex]

%--------------------------------------
\newpage
\section{Extended related work}
\label{sec:appendix:related-work}
%--------------------------------------

\mm{All related work that don't fit in the main paper should go here.}
