# Supplementary material for: LLM2Vec: Large Language Models Are Secretly Powerful Text Encoders
Source: arXiv:2404.05961 source file (2024-08-21)
Supplement: Supplementary file 5 [file ablation_table_appendix.tex]

\begin{table*}[ht]
    \centering
    \small
    \begin{tabular}{lccccccccc}
    \toprule
    \multicolumn{1}{l}{\multirow{2}{*}{\# of datasets $\rightarrow$}} & Retr. & Rerank. & Clust. & PairClass. & Class. & STS & Avg\\
    \multicolumn{1}{l}{}                                & 3     & 2     & 3          & 1      & 3    & 3    & 15  \\
    \midrule
    \multicolumn{1}{l}{medi-ml-miracl bi mean}  & 58.05  & 71.08  & 42.93  &  92.07  & 69.68  & 85.76 & \textbf{66.90} \\
    \midrule
    \multicolumn{9}{l}{\emph{Connections and Pooling}}        \\ \midrule
    \multicolumn{1}{l}{mistral medi-ml-miracl bi eos} & 58.77 & 71.1 & 43.55 & 85.3 & 69.57 & 85.87 & 66.72 \\
    \multicolumn{1}{l}{mistral medi-ml-miracl bi w-mean}  & 57.96 & 70.96 & 42.94 & 92.24 & 69.91 & 85.49 & 66.87 \\ 
    \multicolumn{1}{l}{mistral medi-ml-miracl uni eos}  & 58.35 & 70.62 & 42.76 & 88.96 & 69.52 & 85.87 & 66.65\\ 
    \multicolumn{1}{l}{mistral medi-ml-miracl uni mean}  & 56.81 & 70.55 & 41.48 & 88.91 & 70.72 & 84.82 & 66.1 \\ 
    \multicolumn{1}{l}{mistral medi-ml-miracl uni w-mean}  & 56.81 & 70.53 & 41.42 & 90.15 & 70.79 & 85.42 & 66.3 \\ 
    \midrule
    \multicolumn{9}{l}{\emph{Instruction-tuned}}        \\ \midrule
    \multicolumn{1}{l}{no-instruct medi-ml-miracl bi mean} & 58.28 & 71.71 & 42.82 & 94.2 & 69.26 & 83.14 & 66.54 & \\
    \midrule
    \multicolumn{9}{l}{\emph{Hyperparameters}}        \\ \midrule
    \multicolumn{1}{l}{mistral medi-ml-miracl bi mean lora\_r-8} & 57.92 & 71.03 & 43.4 & 91.42 & 69.69 & 85.6 & 66.89\\
    \multicolumn{1}{l}{mistral medi-ml-miracl bi mean lora\_r-32} & 58.08 & 71.04 & 42.55 & 91.67 & 70.76 & 85.61 & 66.98\\
    \multicolumn{1}{l}{mistral medi-ml-miracl bi mean bs-256} & 58.12 & 70.52 & 42.72 & 83.57 & 69.44 & 84.32 & 65.89\\
    \multicolumn{1}{l}{mistral medi-ml-miracl bi mean bs-512} & 57.55 & 70.5 & 41.77 & 80.79 & 68.57 & 84.36 & 65.24\\
    \midrule
    \multicolumn{9}{l}{\emph{Training Data}}        \\ \midrule
    \multicolumn{1}{l}{mistral medi-eng-miracl bi mean} & 57.41 & 71.09 & 42.55 & 81.44 & 69.42 & 85.21 & 65.83 \\
    \multicolumn{1}{l}{mistral medi bi mean} & 57.6 & 70.61 & 43.24 & 91.57 & 70.11 & 85.27 & 66.76 \\
    \bottomrule
    \end{tabular}
    \caption{Dummy caption for ablation table, all without MLM. mistral-7b: \{uni,bi\}, pool\{mean,eos,weighted\}, \{inst,no-inst\}, bs\{256,512\}, lora{8, 32}. \parishadsuggests{}{This table goes to the appendix and another one with MLM models comes instead.}}
    \label{tab:ablation_results_no_mlm}
\end{table*}
