# Supplementary material for: LLM2Vec: Large Language Models Are Secretly Powerful Text Encoders
Source: arXiv:2404.05961 source file (2024-08-21)
Supplement: Supplementary file 6 [file training_data_ablation_appendix.tex]

\begin{table*}[ht]
    \centering
    \small
    \begin{tabular}{lccccccccc}
    \toprule
    % \multicolumn{1}{l}{\multirow{2}{*}{\# of datasets $\rightarrow$}} & Class. & Clust. & PairClass. & Rerank & Retr. & STS & Summ. & Avg \\
    % \multicolumn{1}{l}{}                                & 12     & 11     & 3          & 4      & 15    & 10  & 1    & 56  \\
    \multicolumn{1}{l}{\multirow{2}{*}{\# of datasets $\rightarrow$}} & Retr. & Rerank. & Clust. & PairClass. & Class. & STS & Avg\\
    \multicolumn{1}{l}{}                                & 3     & 2     & 3          & 1      & 3    & 3    & 15  \\ 
    \midrule
    % \multicolumn{9}{l}{\emph{Training Data}}        \\ \cmidrule{1-1}
    \multicolumn{1}{l}{medi-ml-miracl}  & 58.05  & 71.08  & 42.93  &  92.07  & 69.68  & 85.76 & \textbf{66.90} \\
    \multicolumn{1}{l}{medi-eng-miracl} & 57.41 & 71.09 & 42.55 & 81.44 & 69.42 & 85.21 & 65.83\\
    \multicolumn{1}{l}{medi} & 57.6 & 70.61 & 43.24 & 91.57 & 70.11 & 85.27 & 66.76\\
    \bottomrule
    \end{tabular}
    \caption{Ablation study of the impact of training data on Mistral-7B on MTEB benchmark (bi-mean Mistral-7b with no MLM training).}
    \label{tab:training-data-ablation}
\end{table*}
